# Supplementary material for: Rapid and Precise Topological Comparison with Merge Tree Neural Networks
Source: arXiv:2404.05879 source file (2024-10-04)
Supplement: Supplementary file 1 [file appendix.tex]

\section{Appendices}
\label{sec:appendix}
