# Supplementary material for: Rapid and Precise Topological Comparison with Merge Tree Neural Networks
Source: arXiv:2404.05879 source file (2024-10-04)
Supplement: Supplementary file 2 [file supplemental.tex]

%\section*{Supplemental Materials}
%\label{sec:supplemental_materials}

%Python implementation url here. 
